# Supplementary material for: Self-explaining variational posterior distributions for Gaussian Process models
Source: arXiv:2109.03708 source file (2021-09-08)
Supplement: Supplementary file 1 [file figures.tex]

\begin{figure}[!h]
\centering
\begin{subfigure}{.5\textwidth}
  \centering
  \includegraphics[width=1.\linewidth]{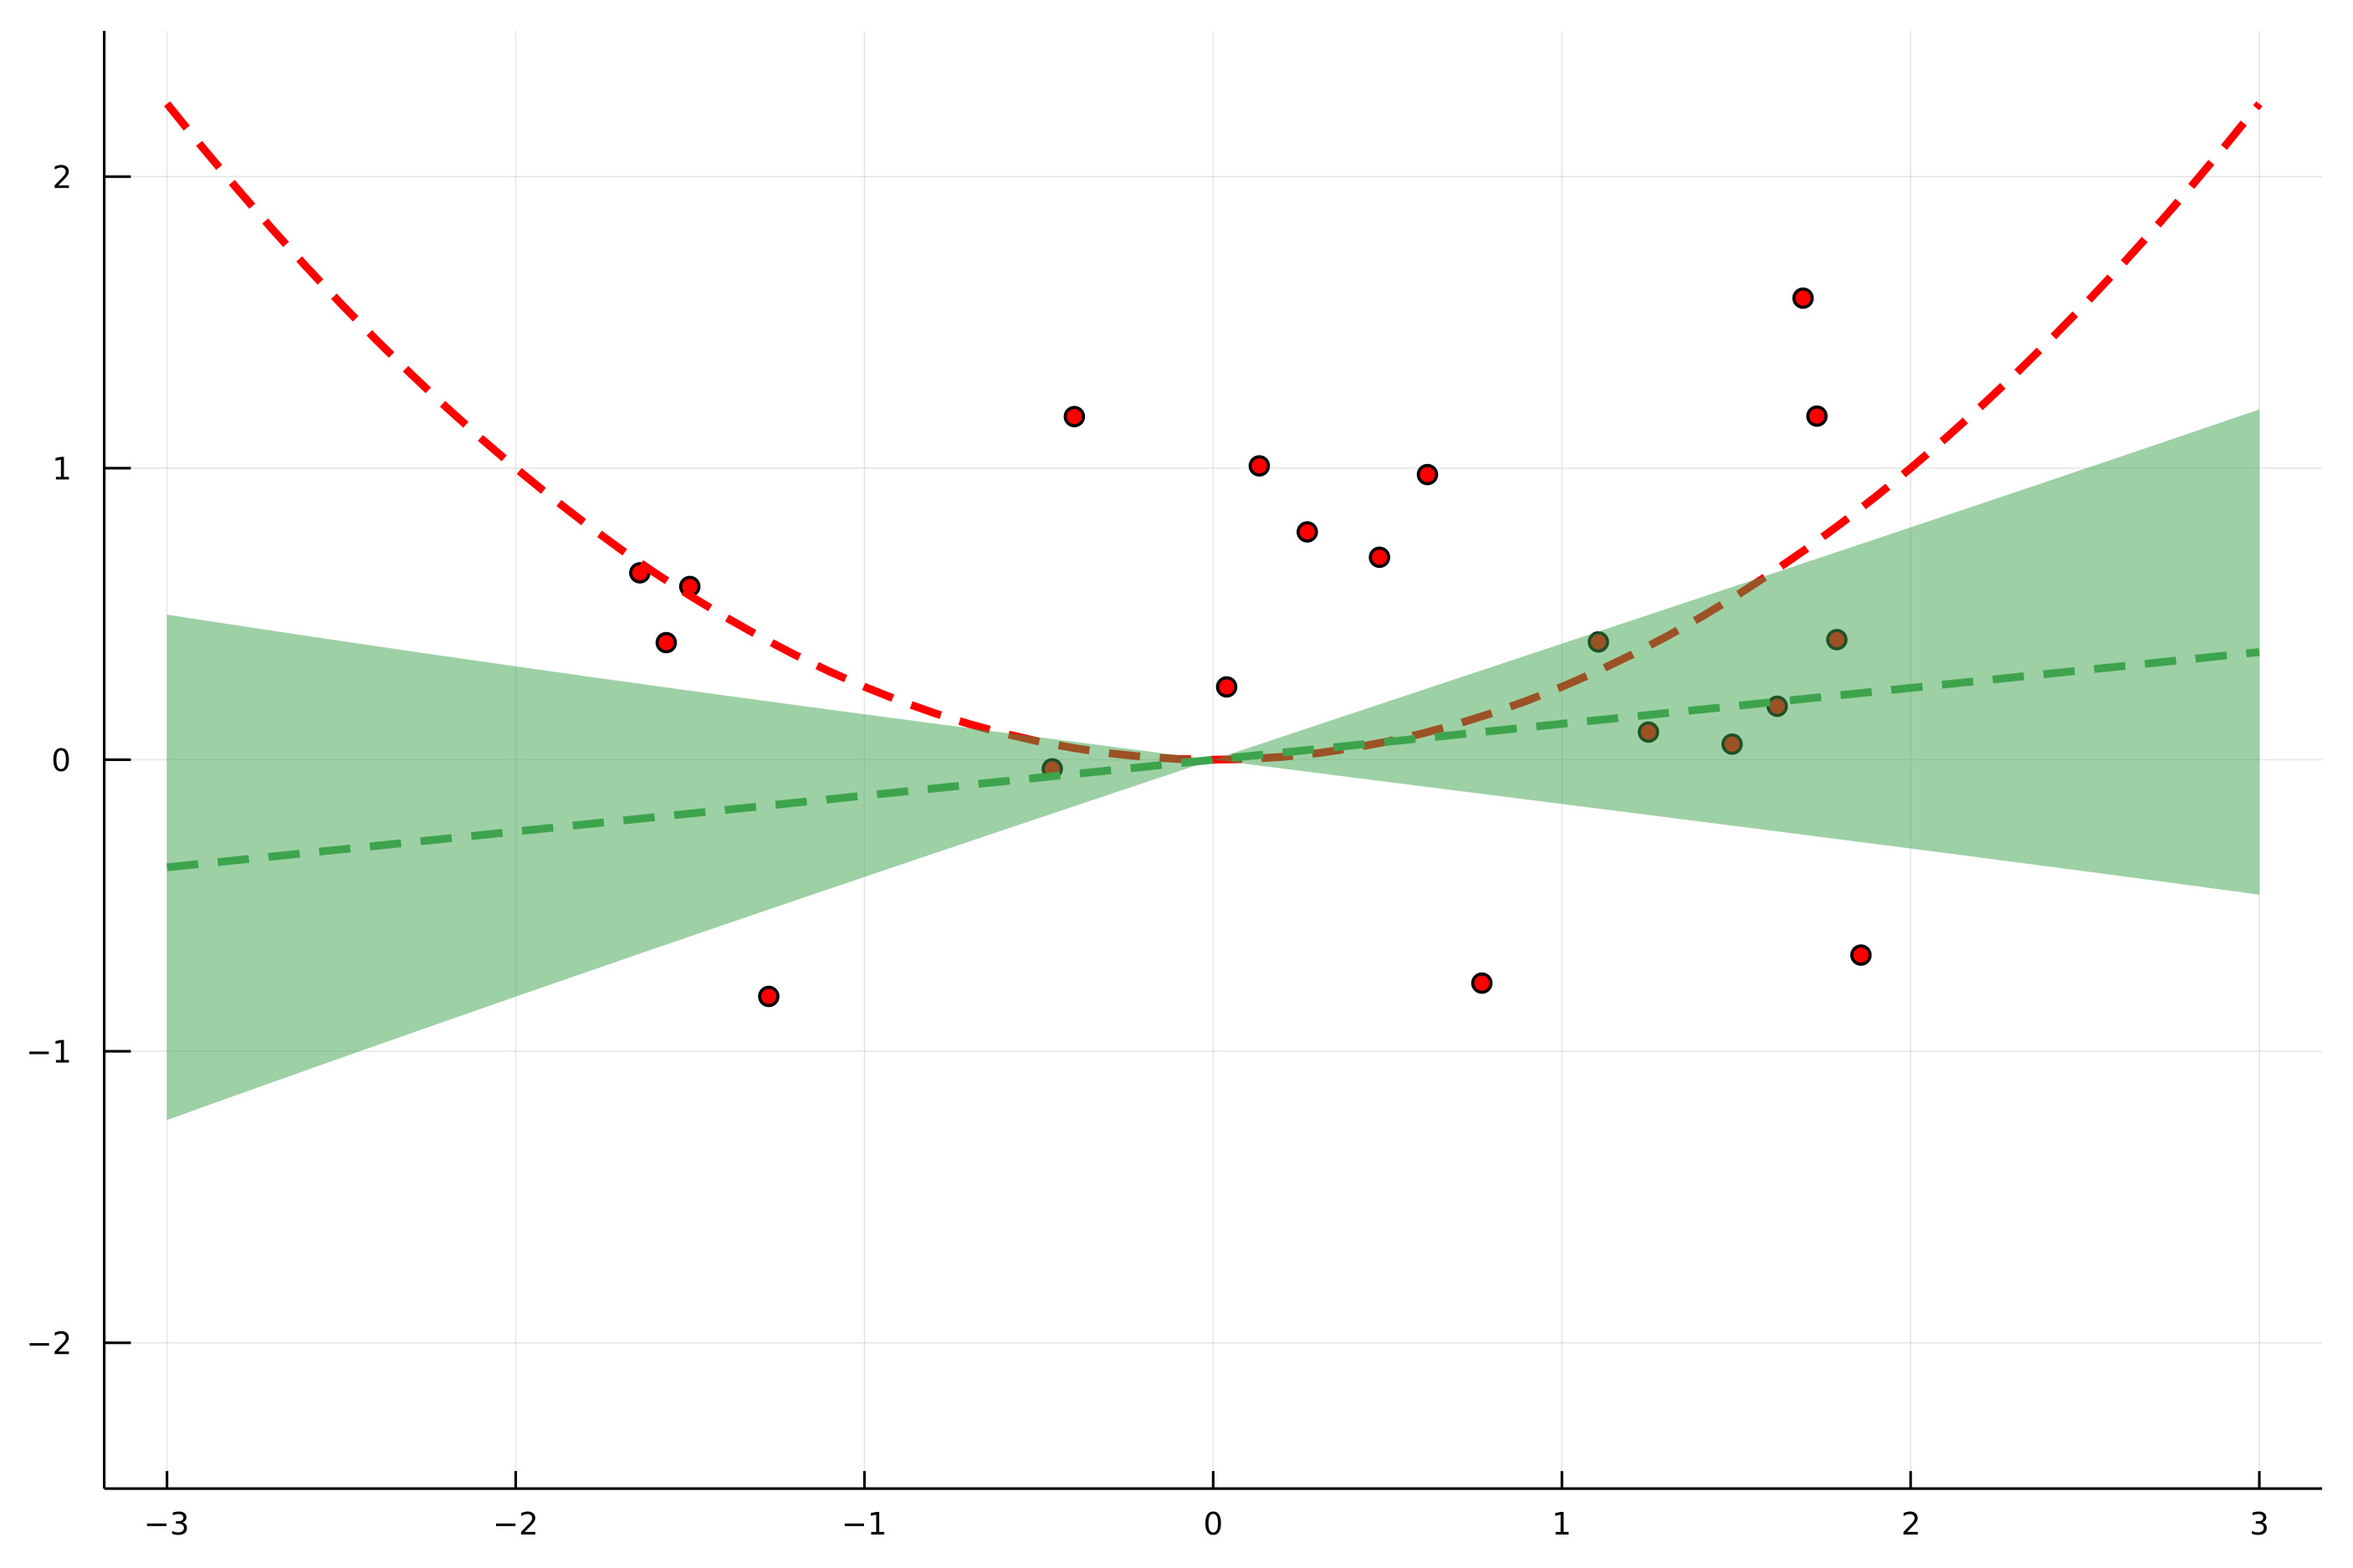}
  \label{fig:model1:sub1}
\end{subfigure}%
\begin{subfigure}{.5\textwidth}
  \centering
  \includegraphics[width=1.\linewidth]{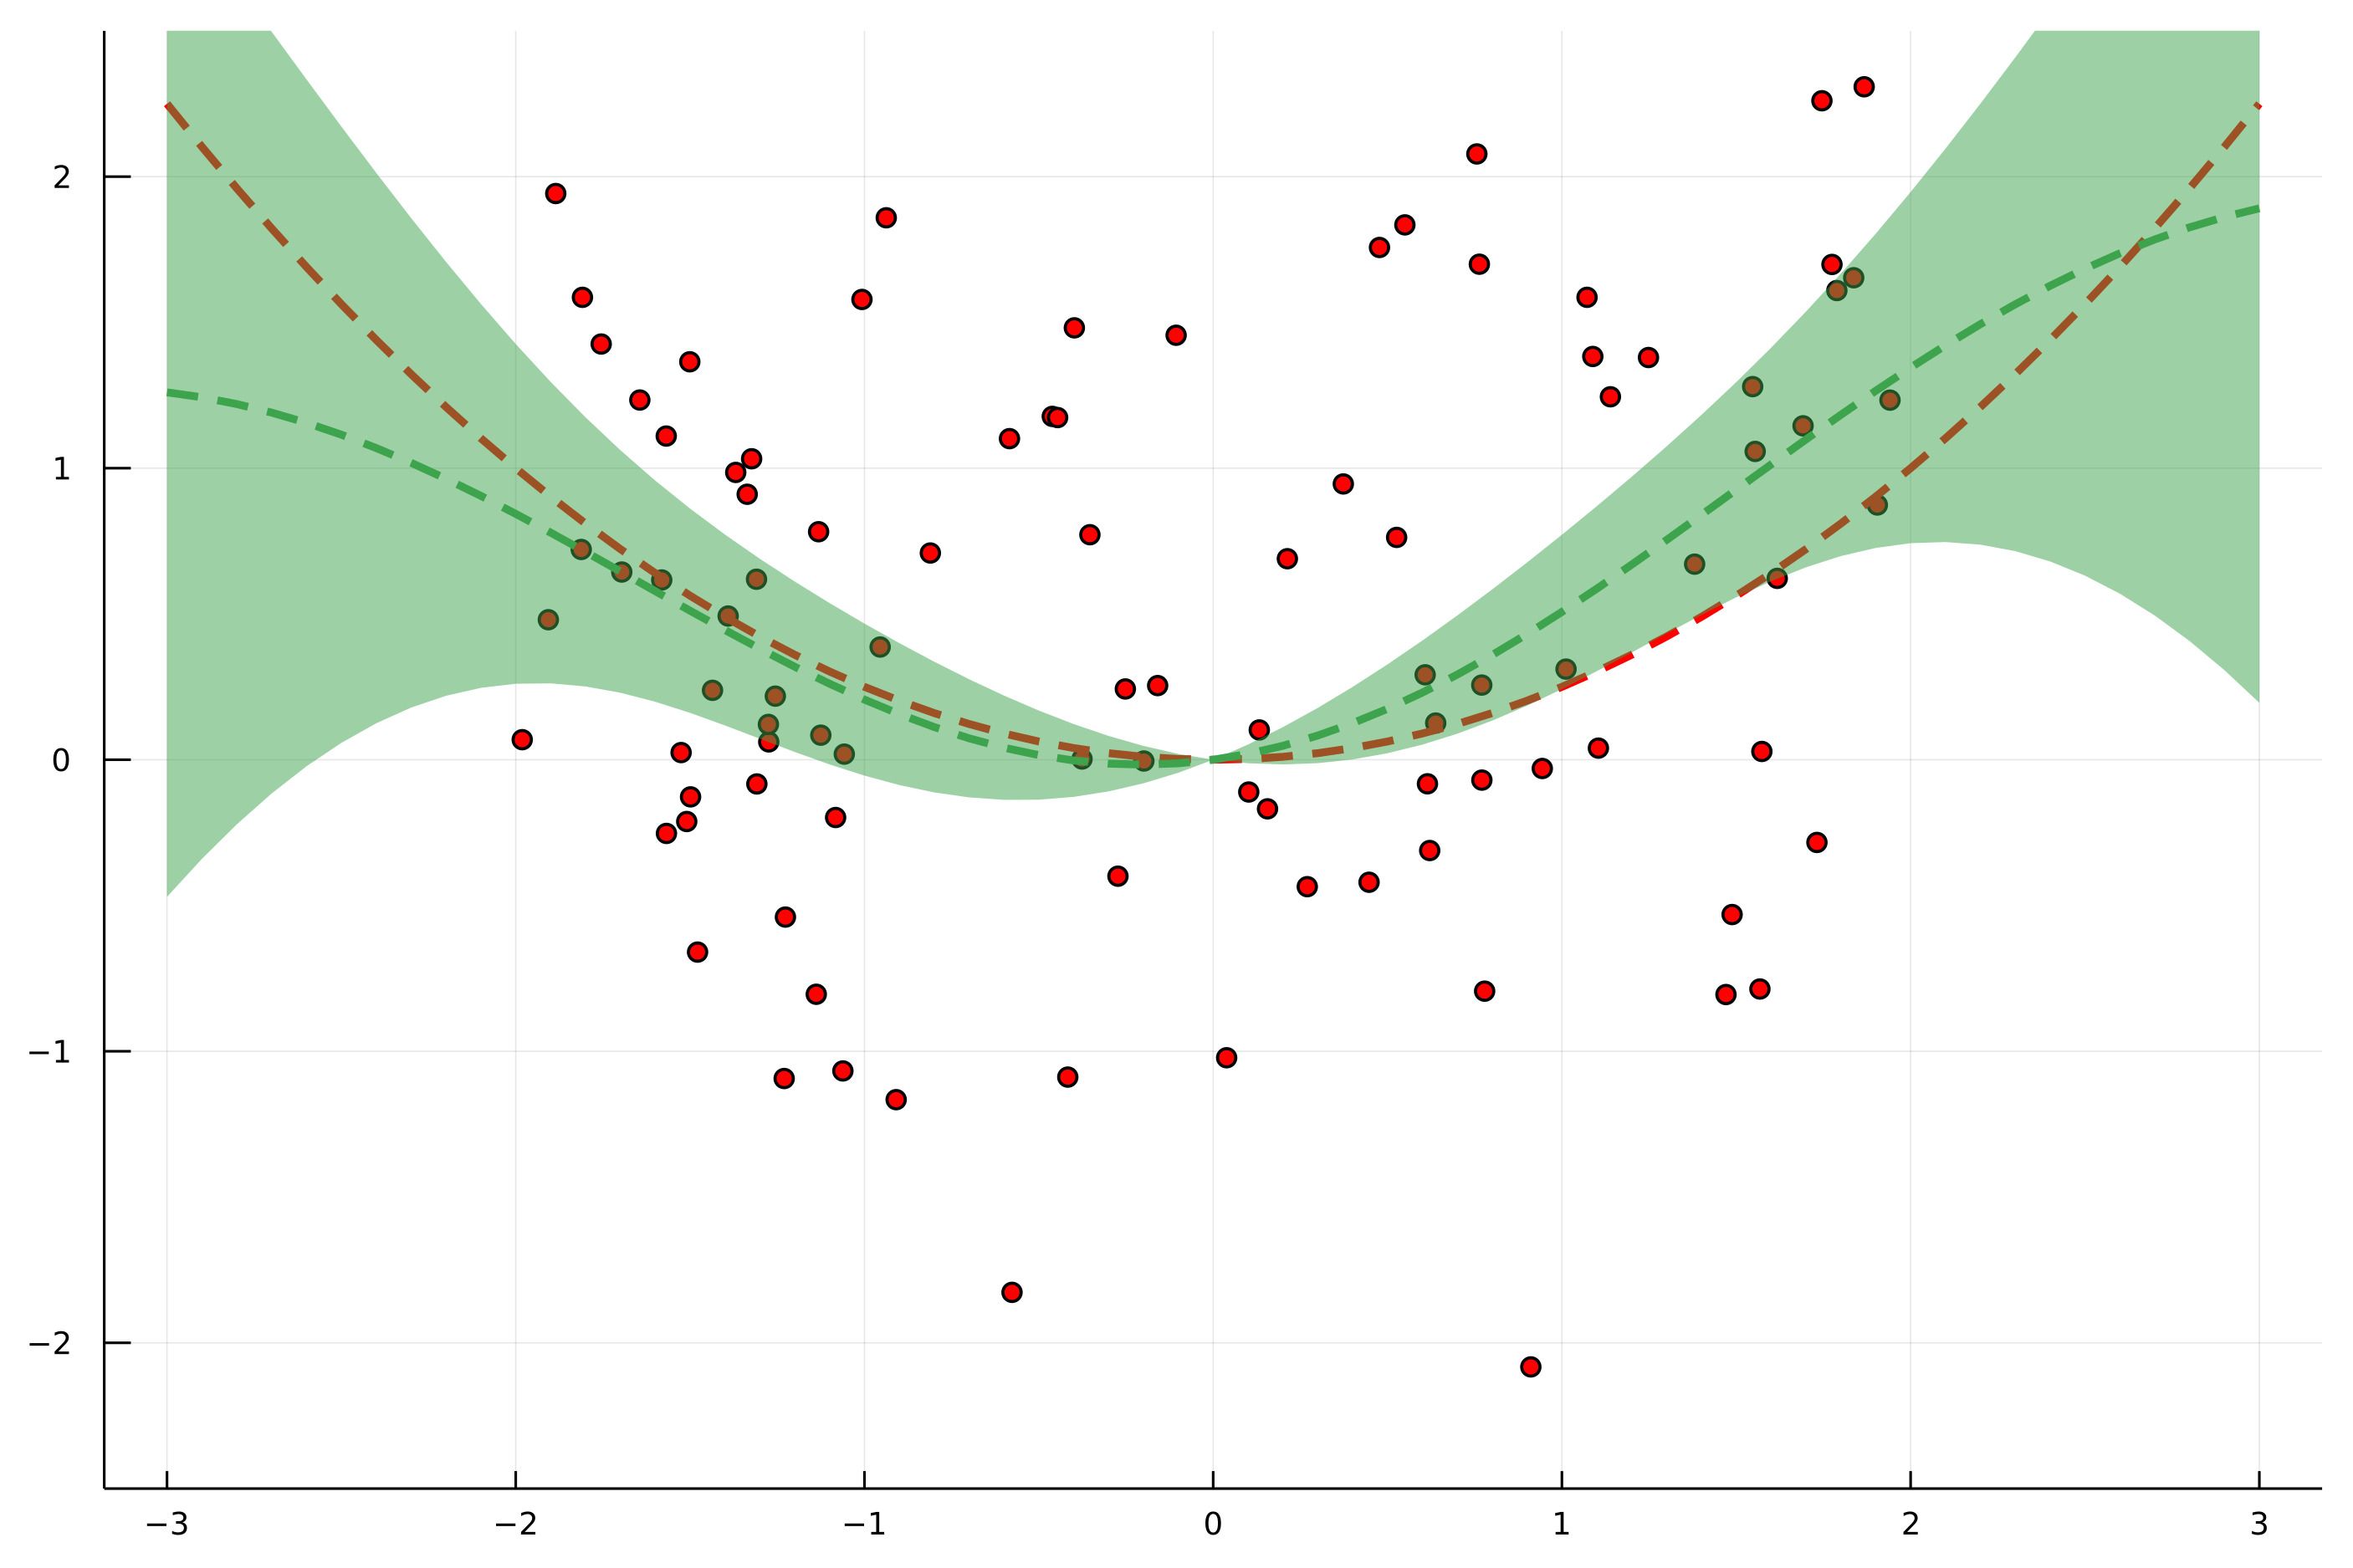}
  \label{fig:model1:sub2}
\end{subfigure}
\caption{Model variant $4.1$ - posterior distribution (mean plus two standard deviations; green line plus interval), mean generating process (red) and sampled datapoints (red dots) for $n_1=20$ observations (left) and $n_2=100$ observations (right)}
\label{fig:model1}
\end{figure}

\begin{figure}[!h]
\centering
\begin{subfigure}{.5\textwidth}
  \centering
  \includegraphics[width=1.\linewidth]{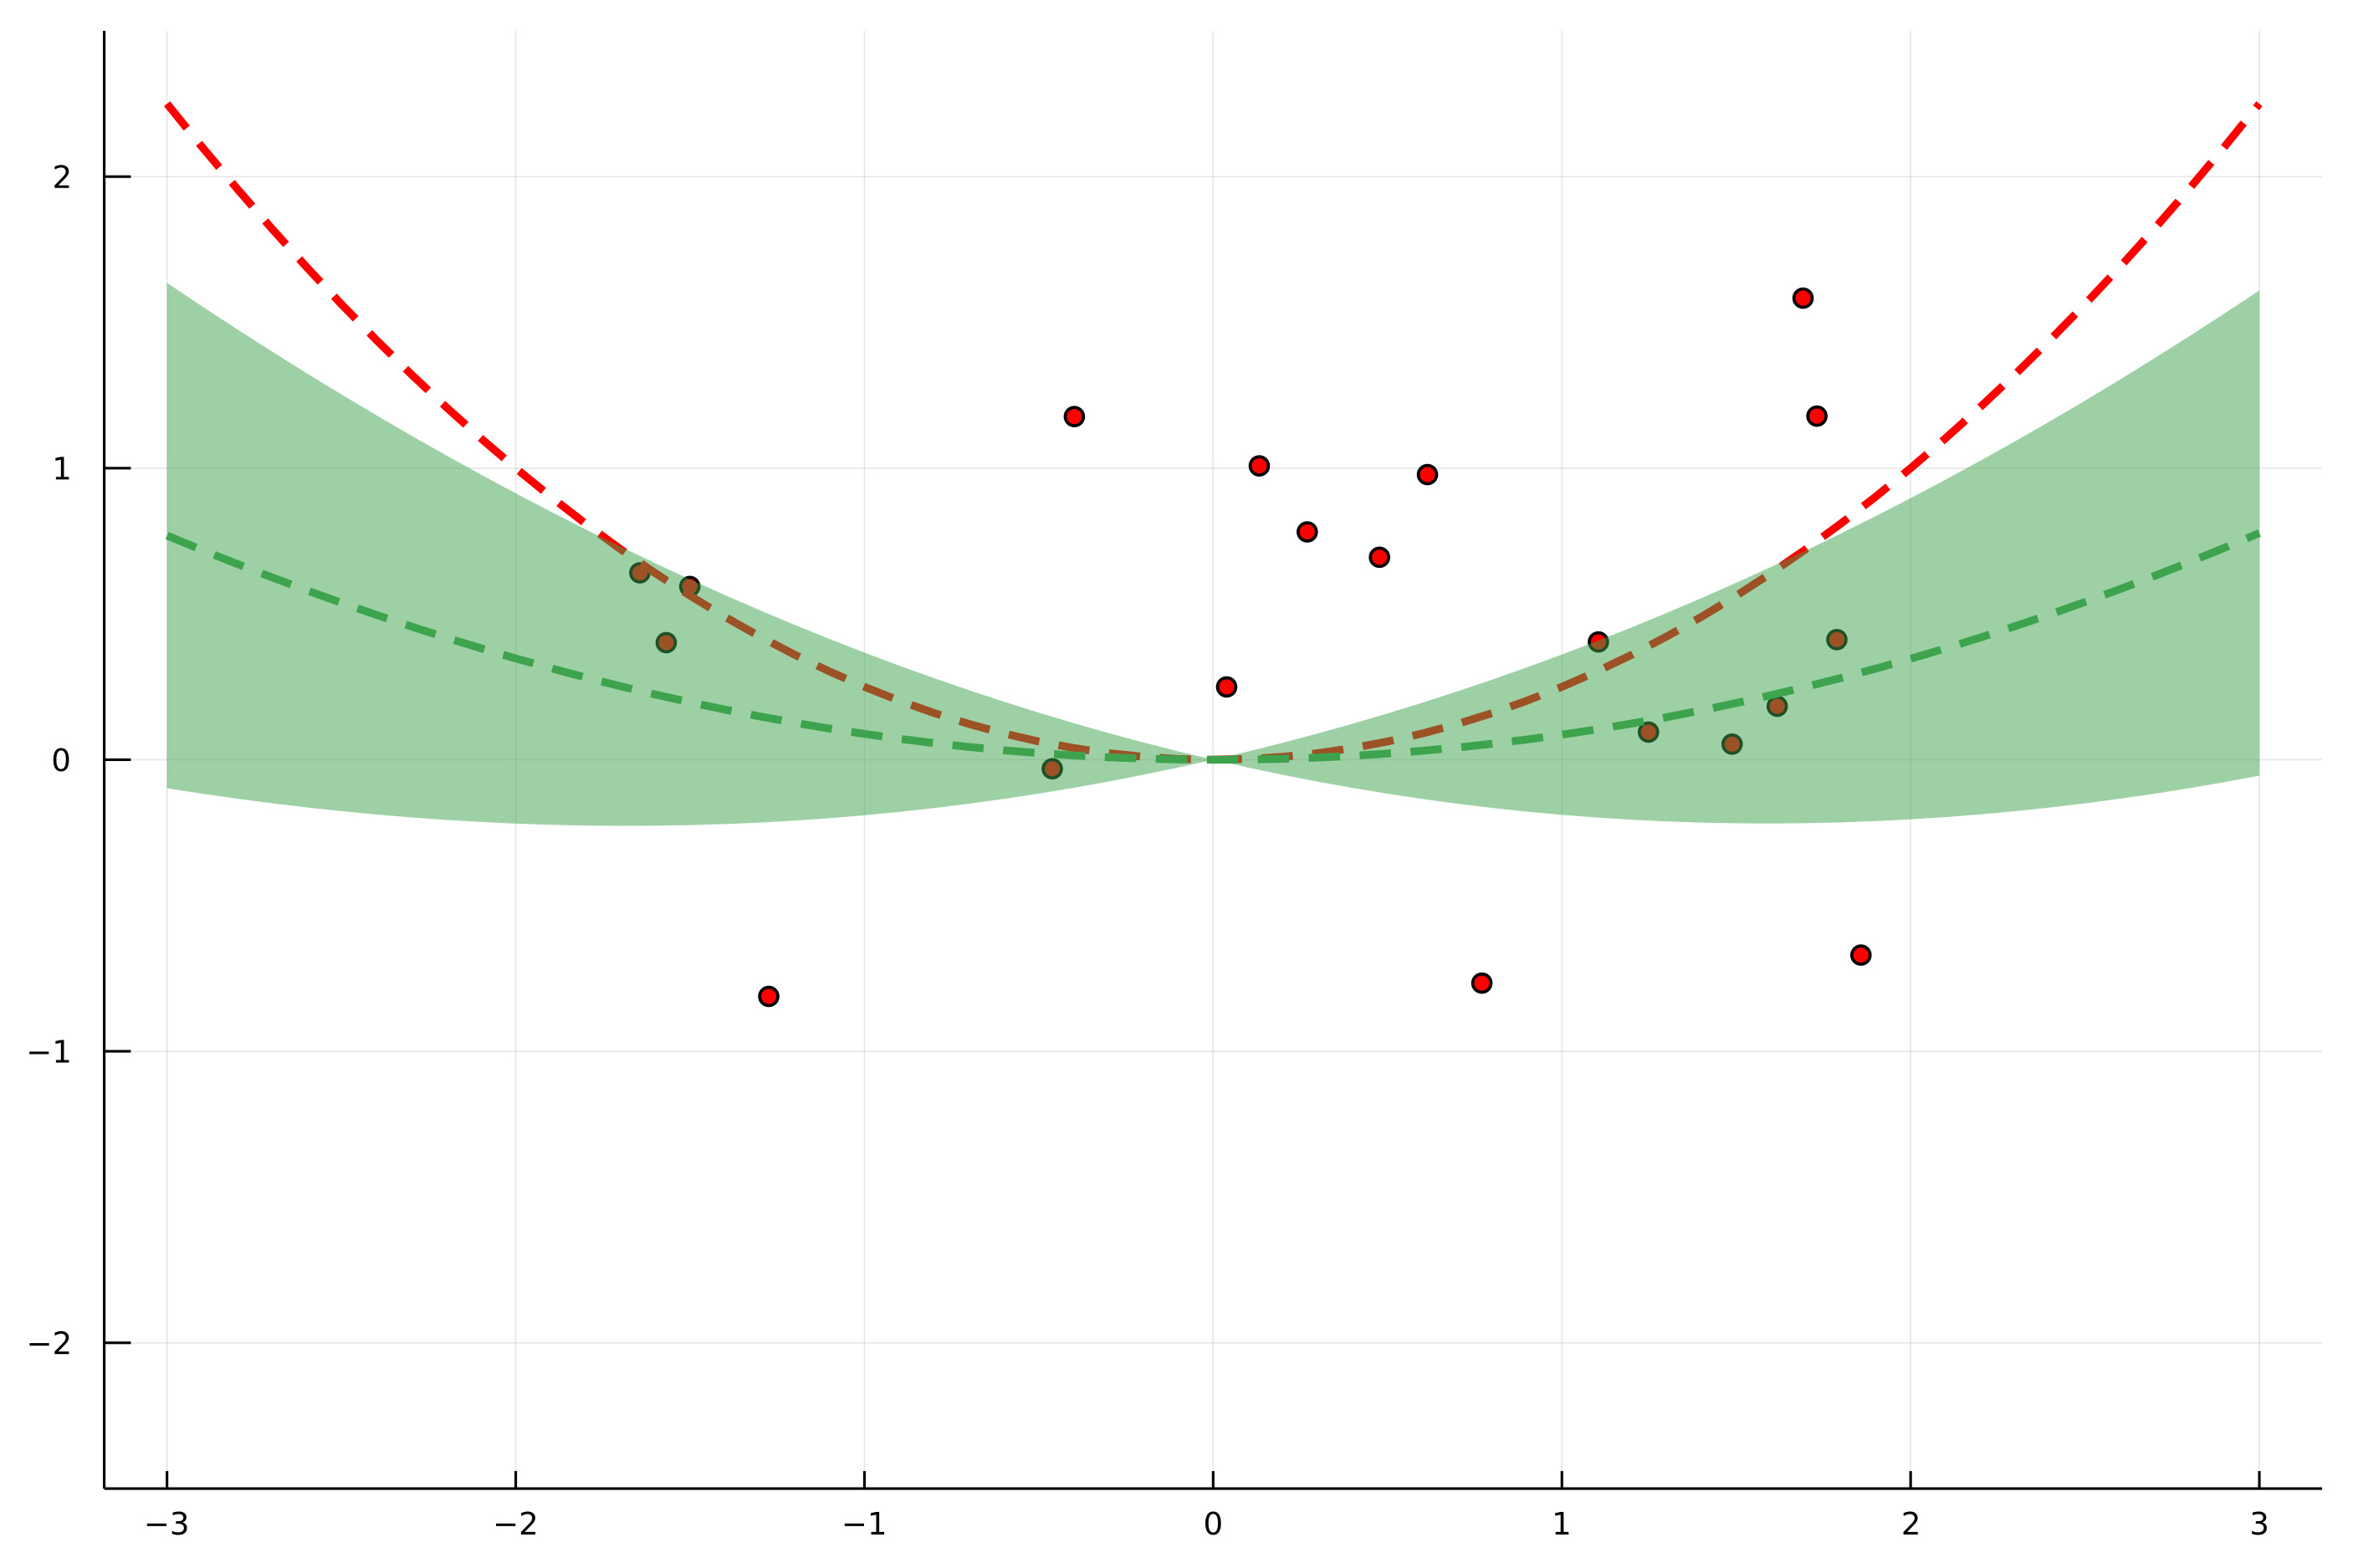}
  \label{fig:model1:sub1}
\end{subfigure}%
\begin{subfigure}{.5\textwidth}
  \centering
  \includegraphics[width=1.\linewidth]{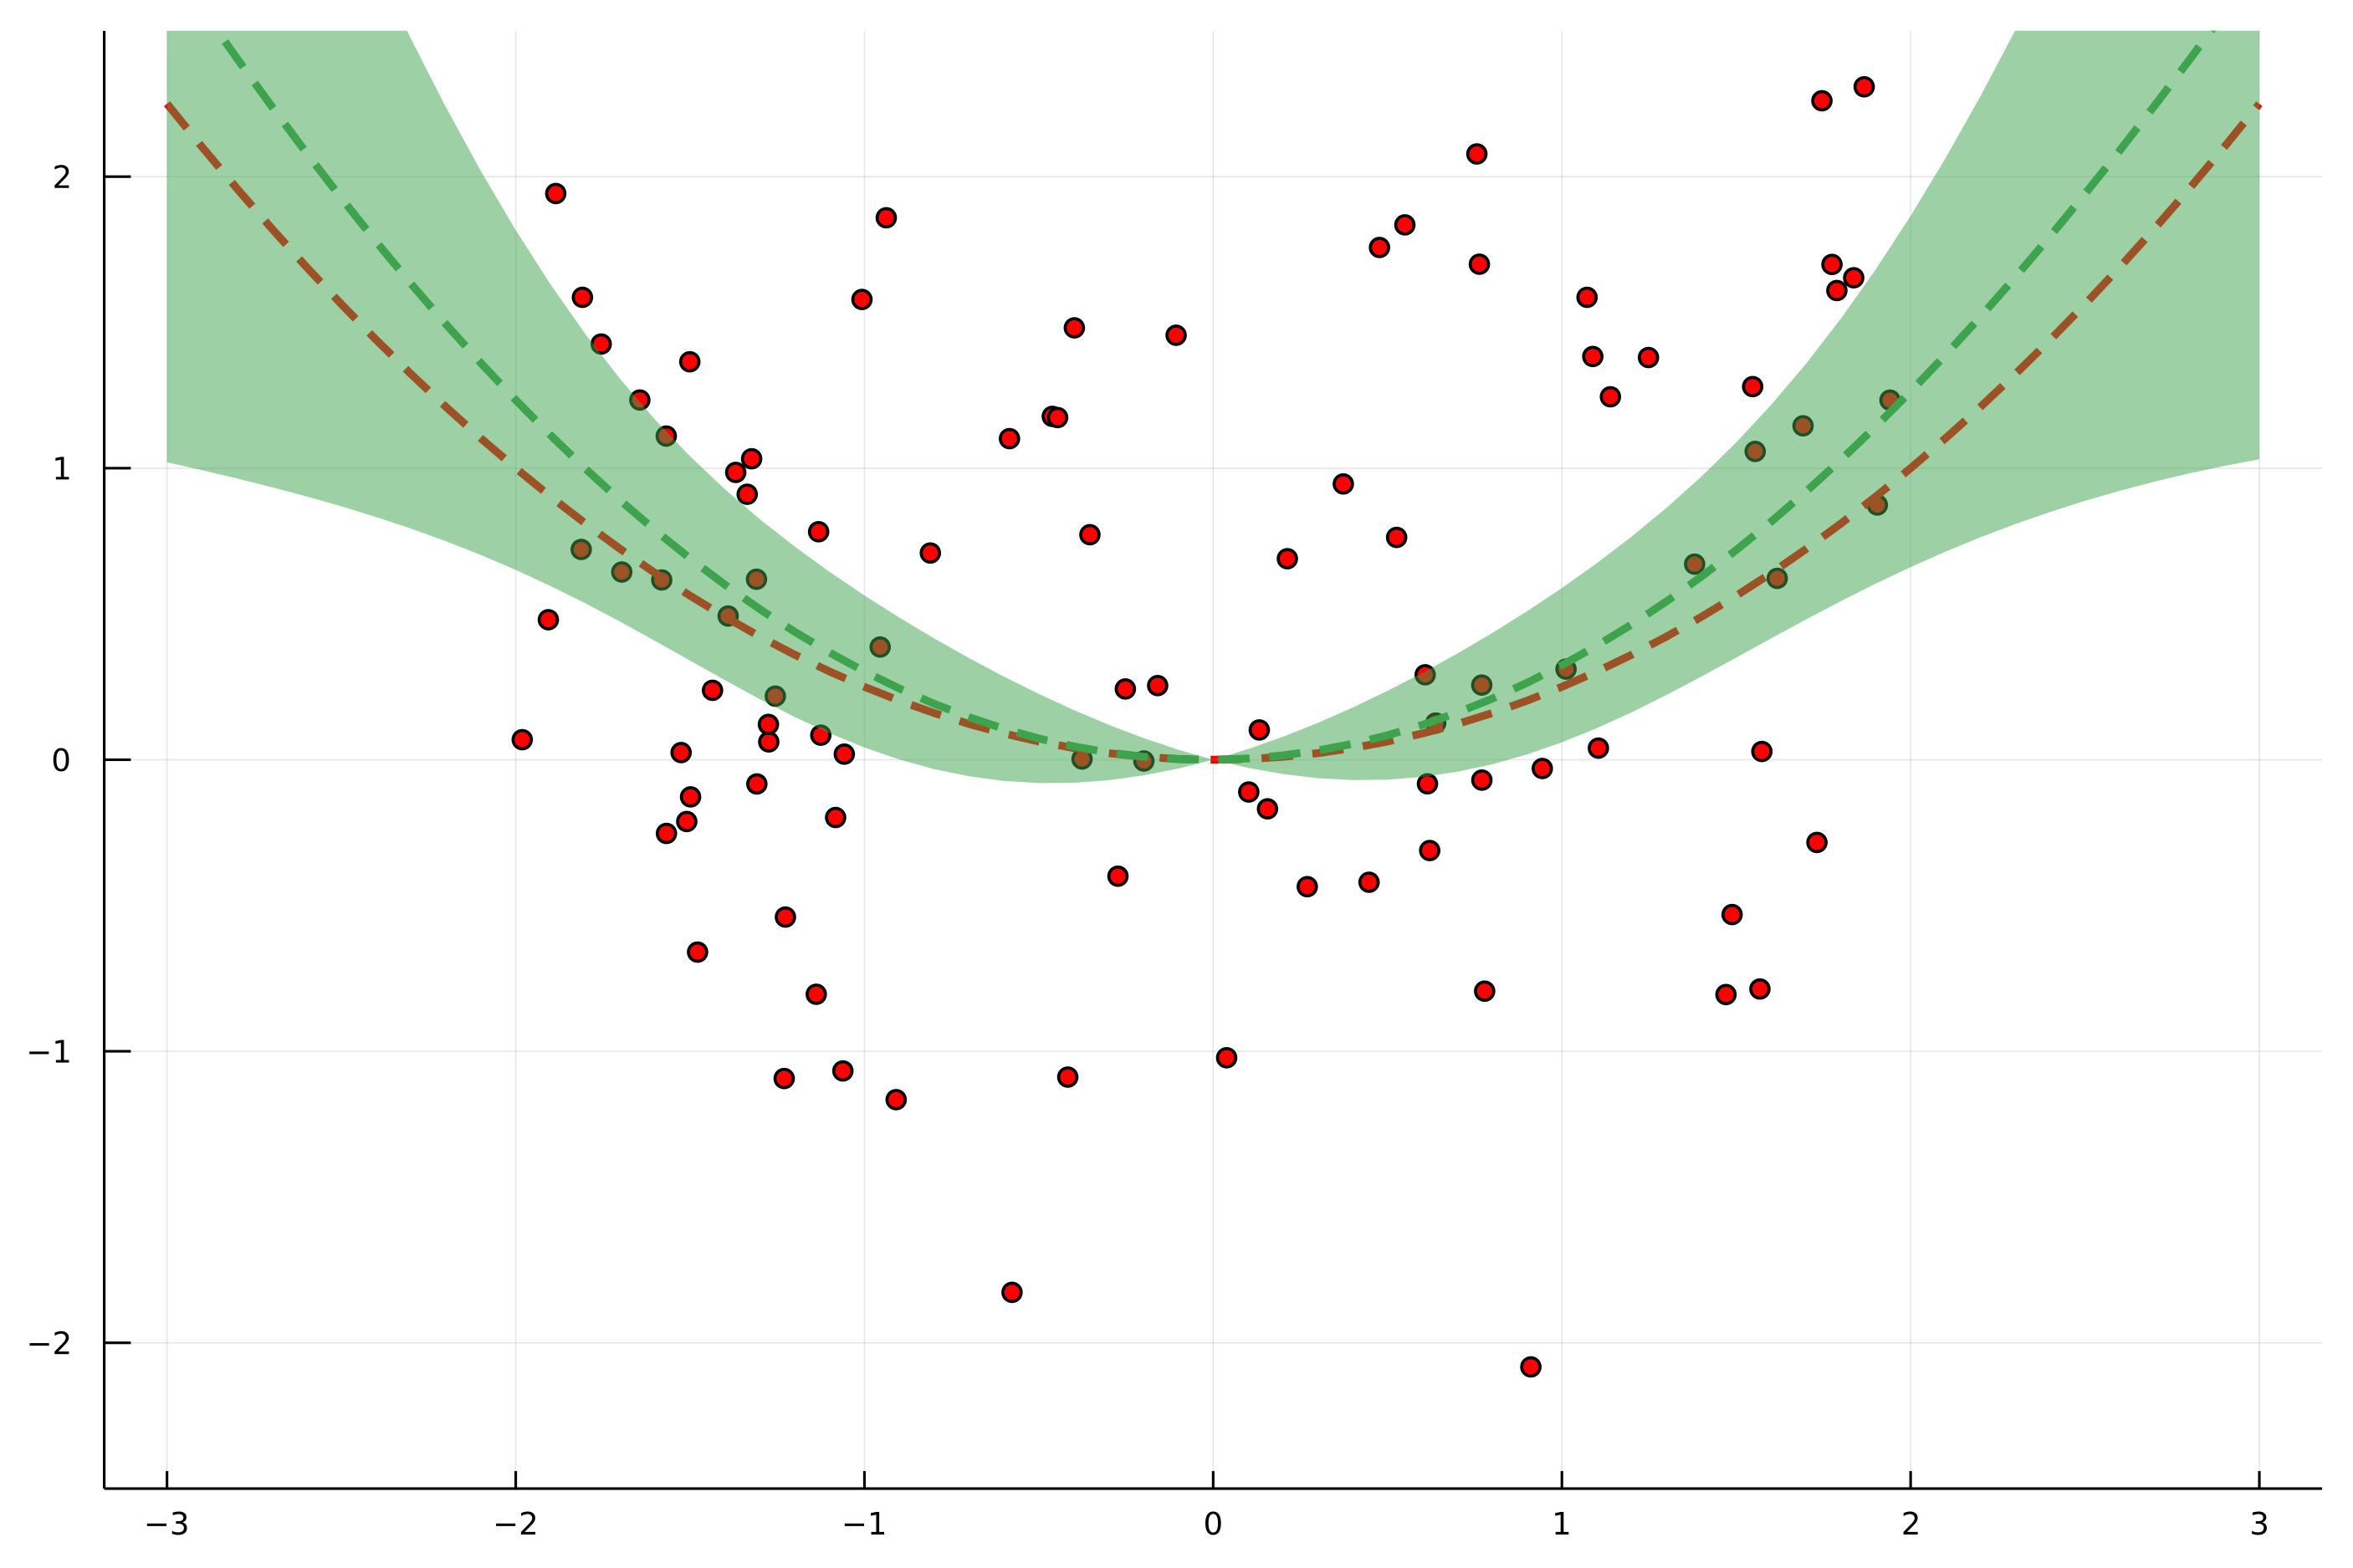}
  \label{fig:model1:sub2}
\end{subfigure}
\caption{Model variant $4.2$ - posterior distribution (mean plus two standard deviations; green line plus interval), mean generating process (red) and sampled datapoints (red dots) for $n_1=20$ observations (left) and $n_2=100$ observations (right)}
\label{fig:model1}
\end{figure}

\begin{figure}[!h]
\centering
\begin{subfigure}{.5\textwidth}
  \centering
  \includegraphics[width=1.\linewidth]{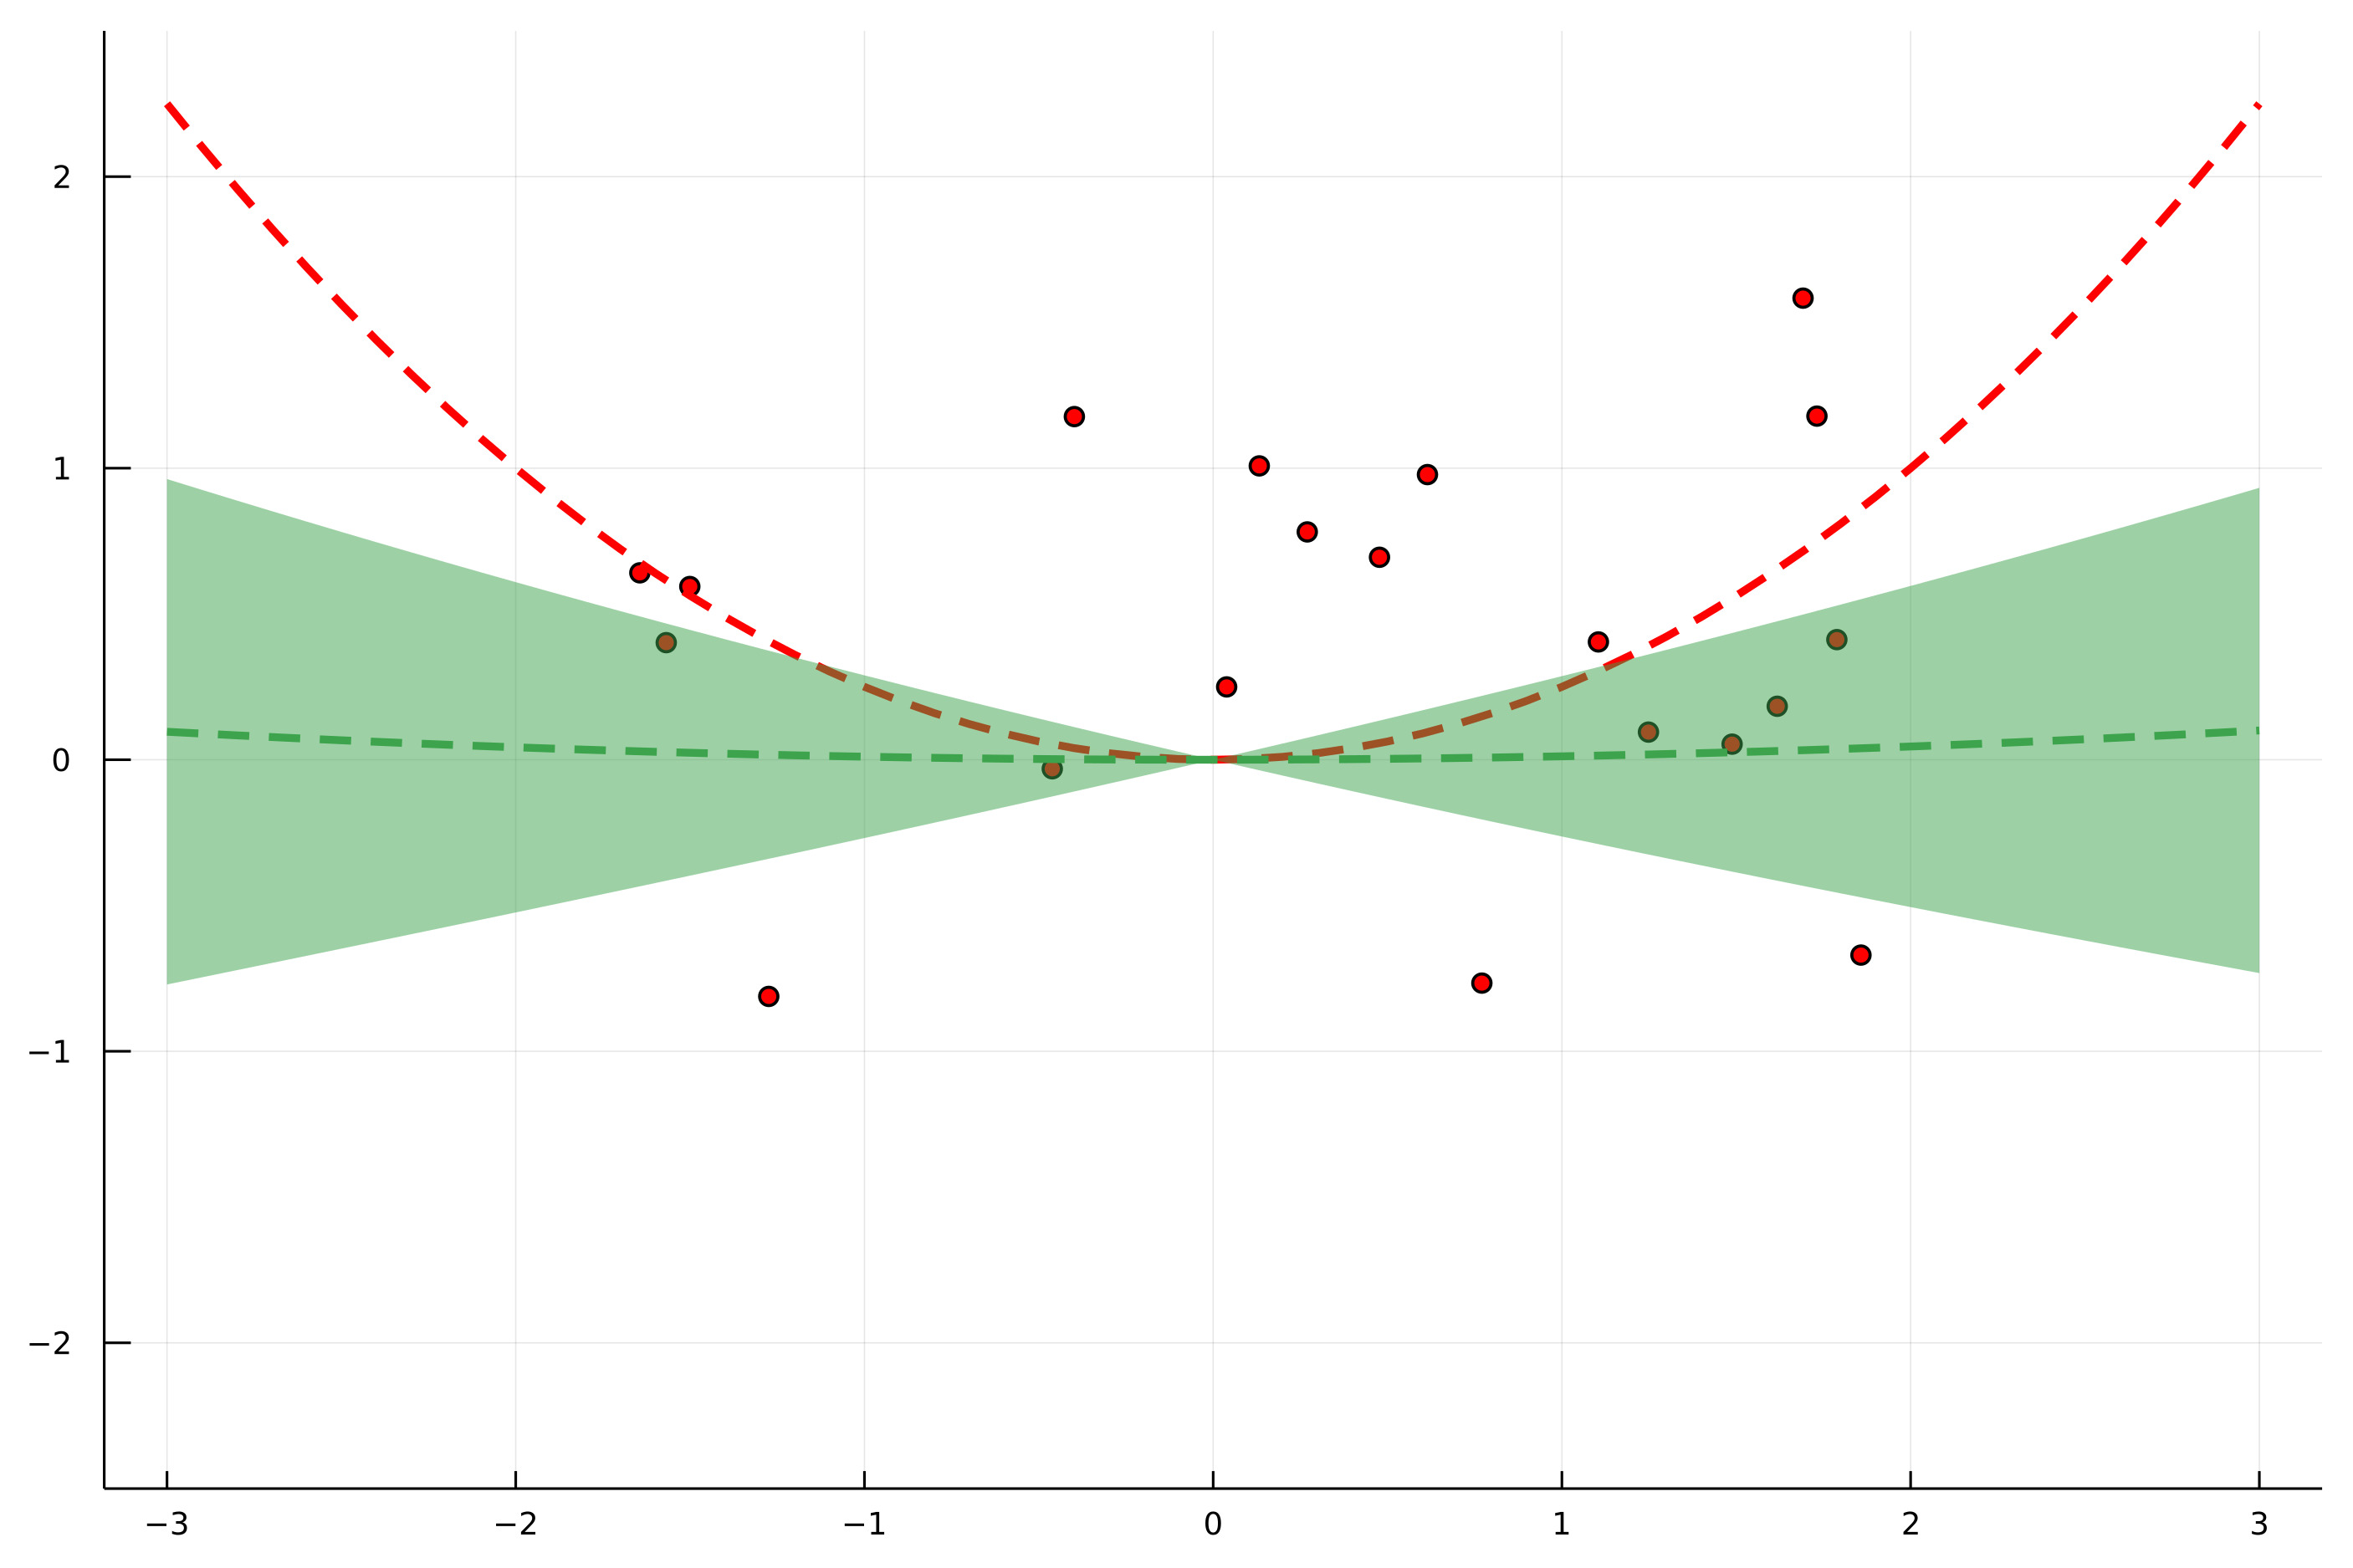}
  \label{fig:model1:sub1}
\end{subfigure}%
\begin{subfigure}{.5\textwidth}
  \centering
  \includegraphics[width=1.\linewidth]{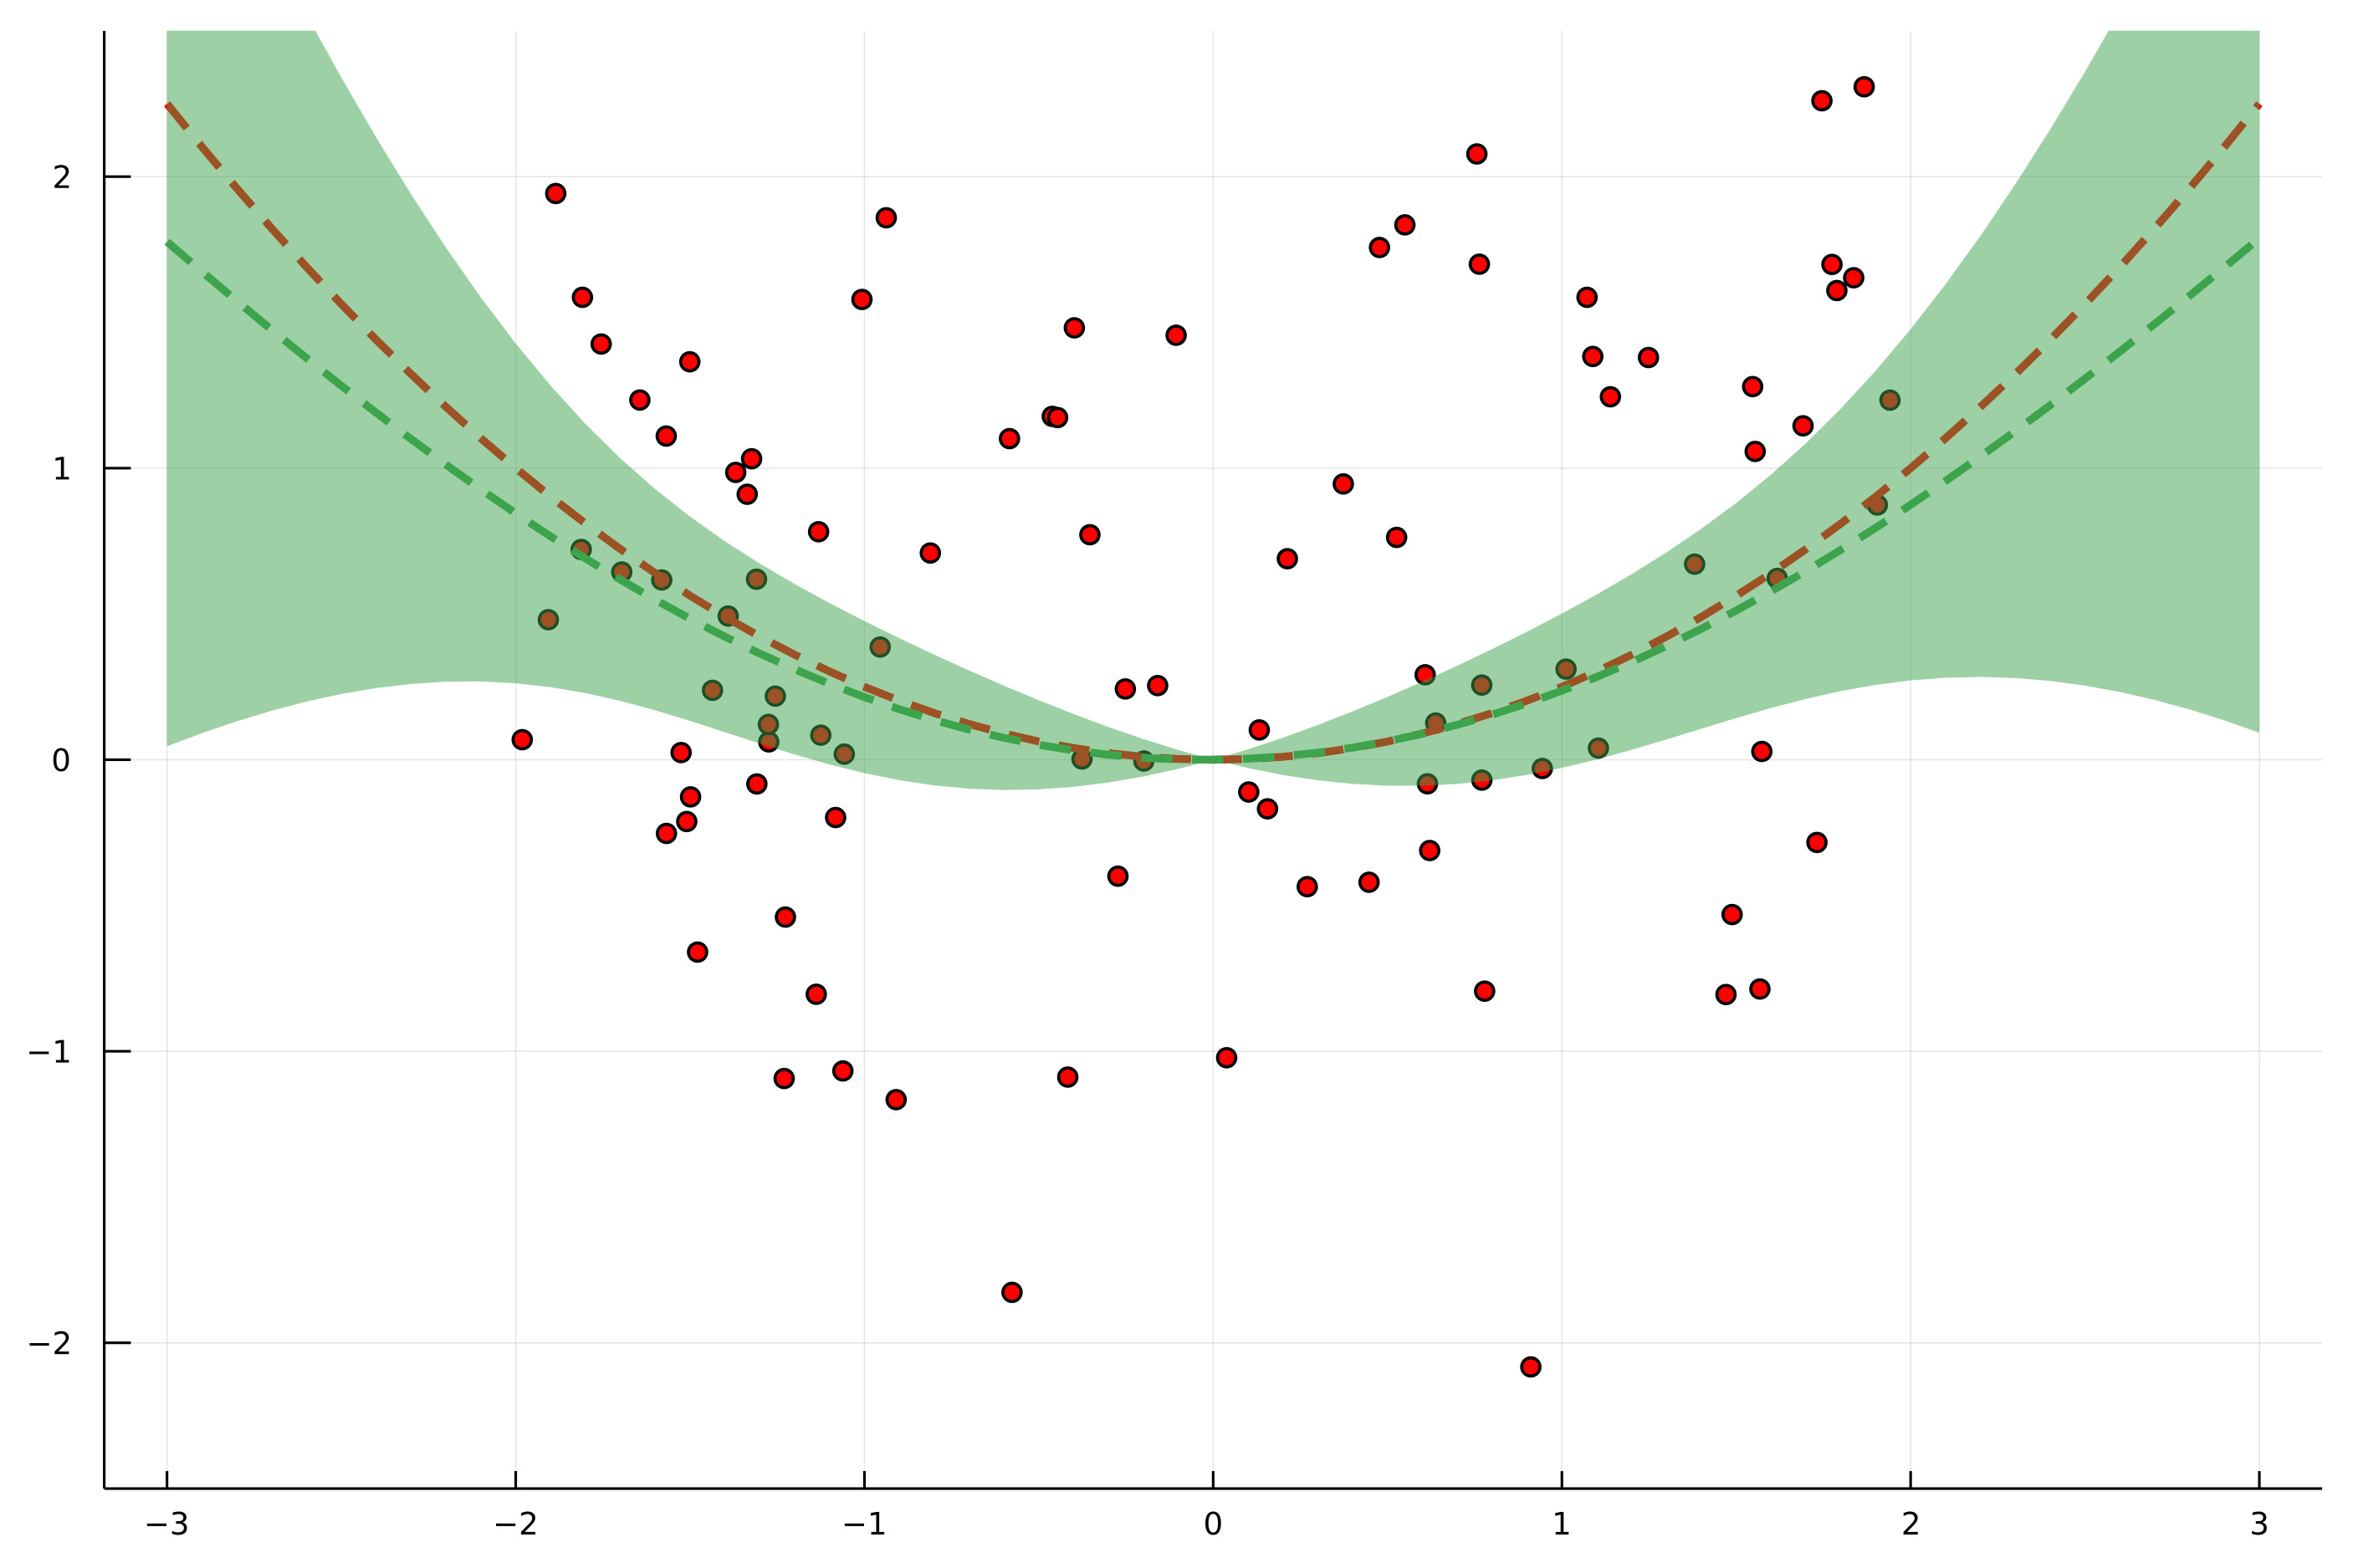}
  \label{fig:model1:sub2}
\end{subfigure}
\caption{Model variant $4.3$ - posterior distribution (mean plus two standard deviations; green line plus interval), mean generating process (red) and sampled datapoints (red dots) for $n_1=20$ observations (left) and $n_2=100$ observations (right)}
\label{fig:model1}
\end{figure}

\begin{figure}[!h]
\centering
\begin{subfigure}{.5\textwidth}
  \centering
  \includegraphics[width=1.\linewidth]{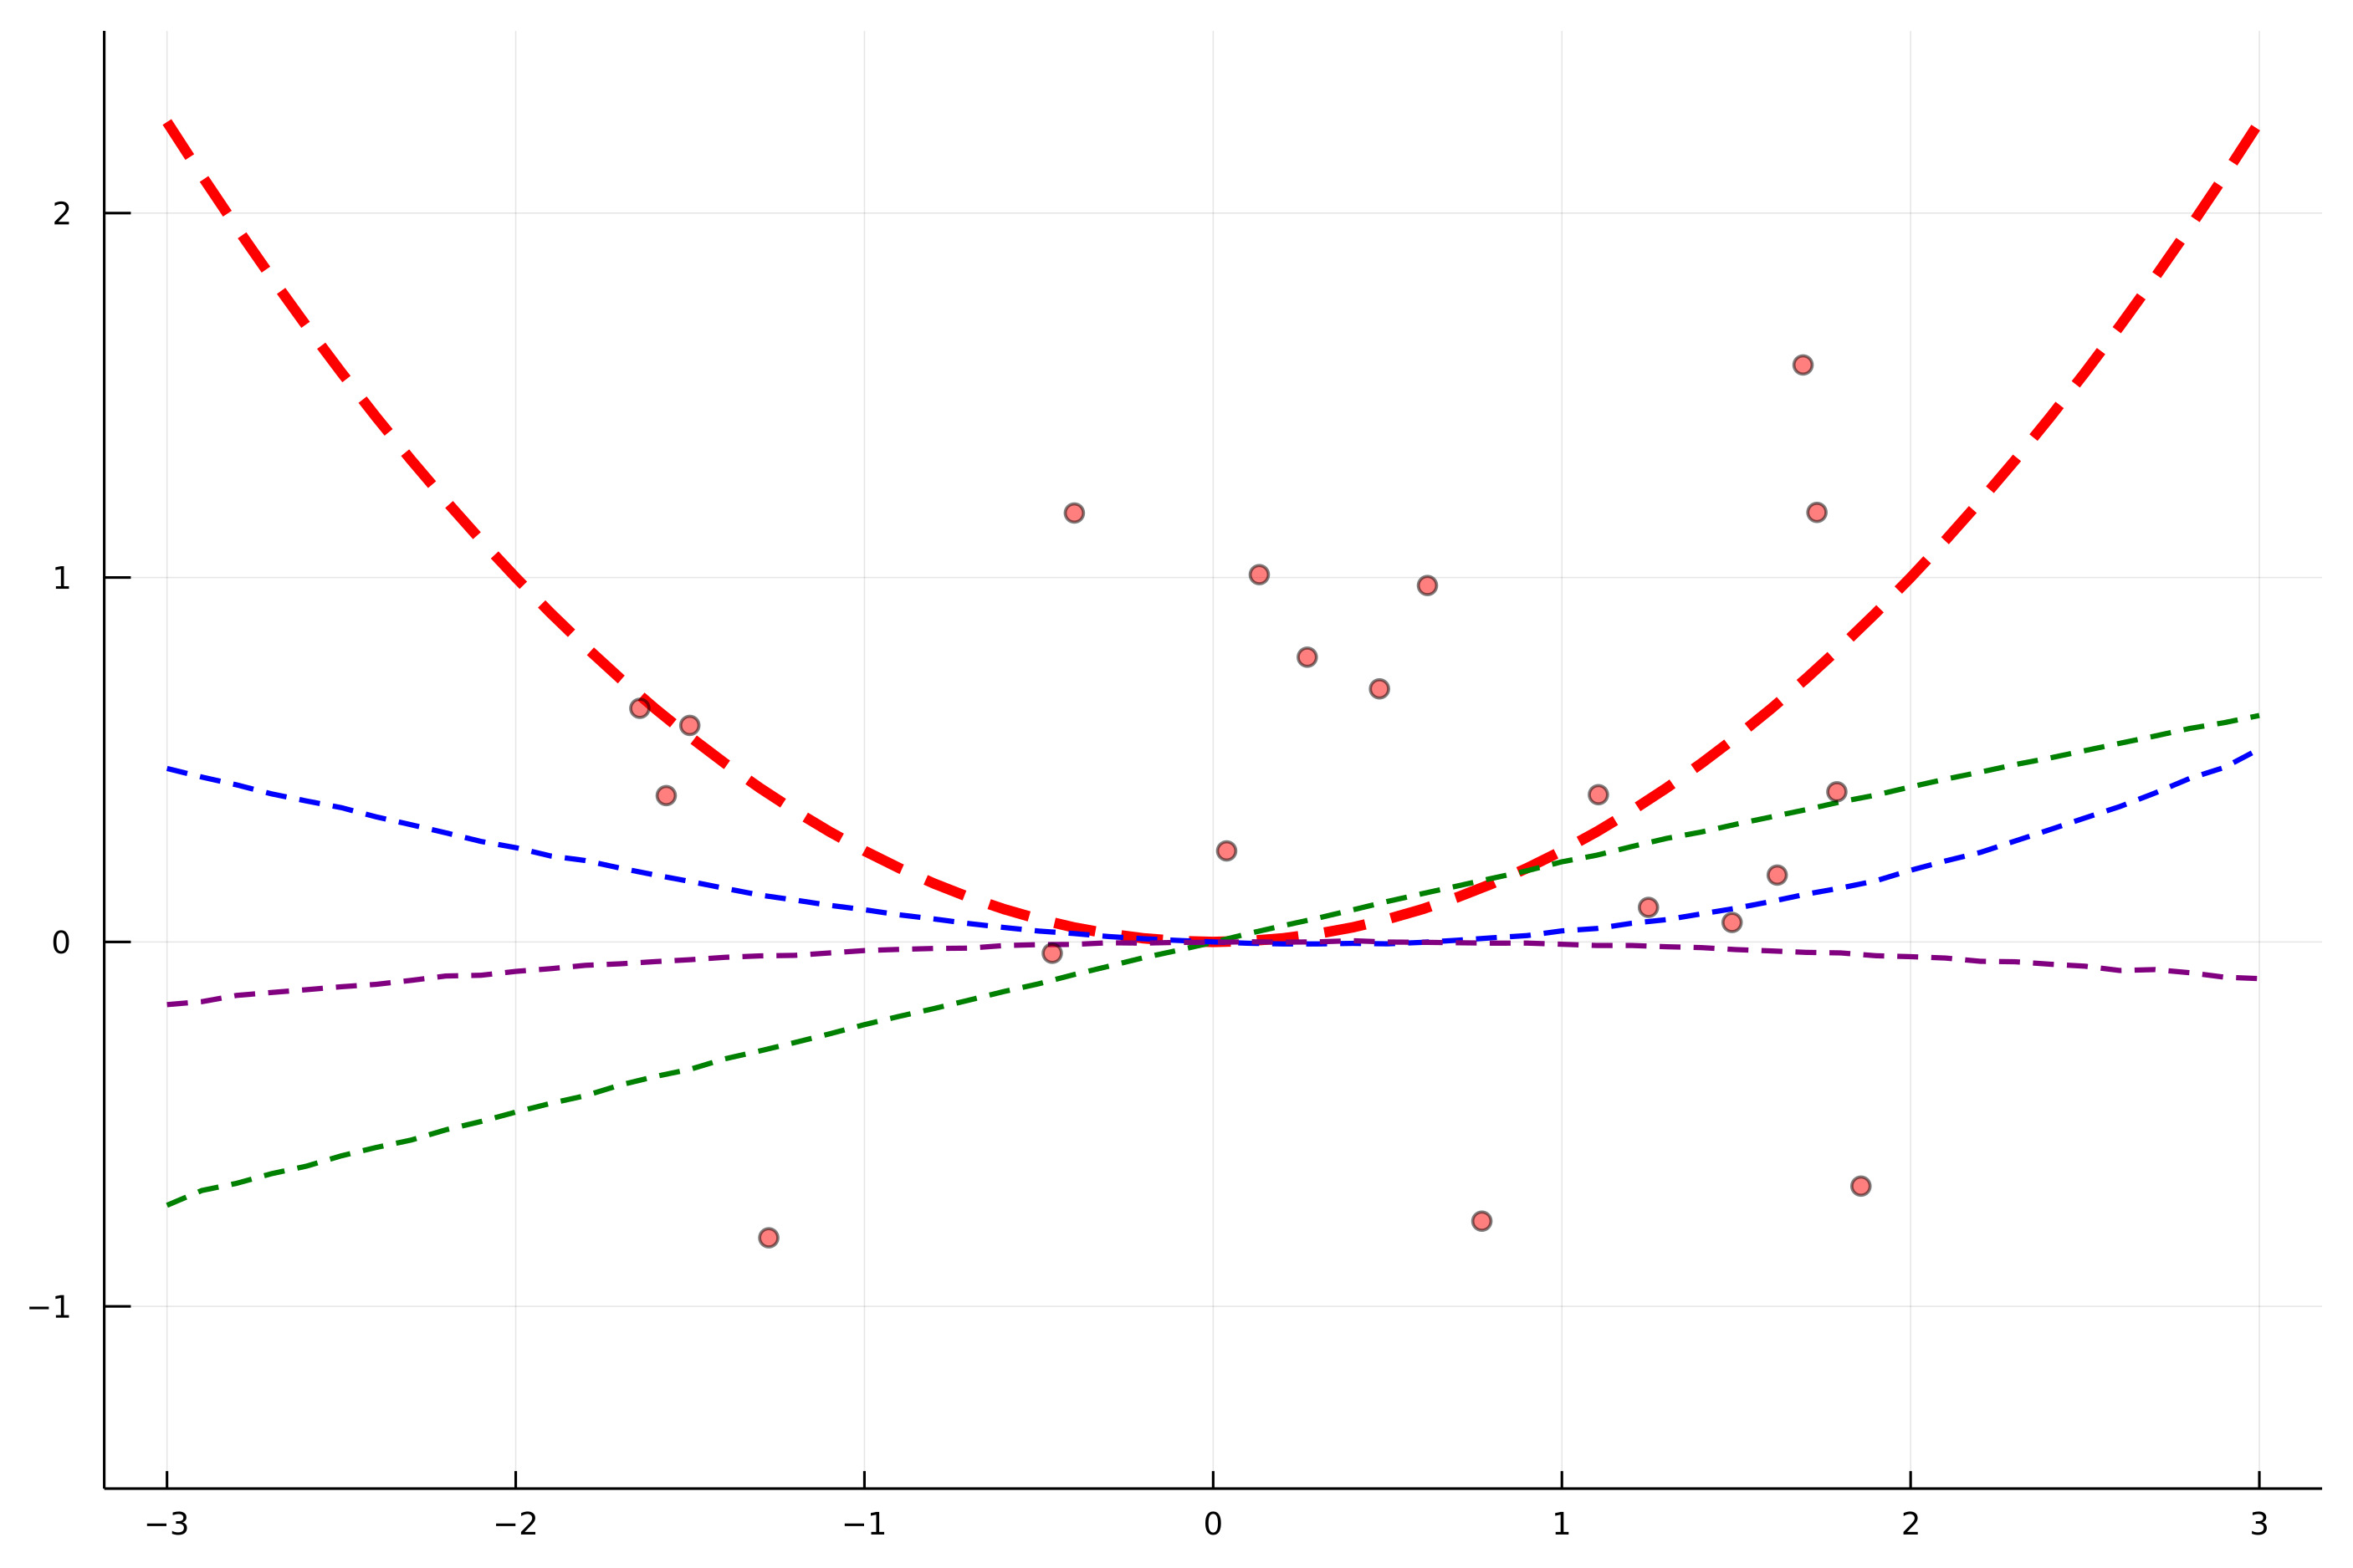}
  \label{fig:model1:sub1}
\end{subfigure}%
\begin{subfigure}{.5\textwidth}
  \centering
  \includegraphics[width=1.\linewidth]{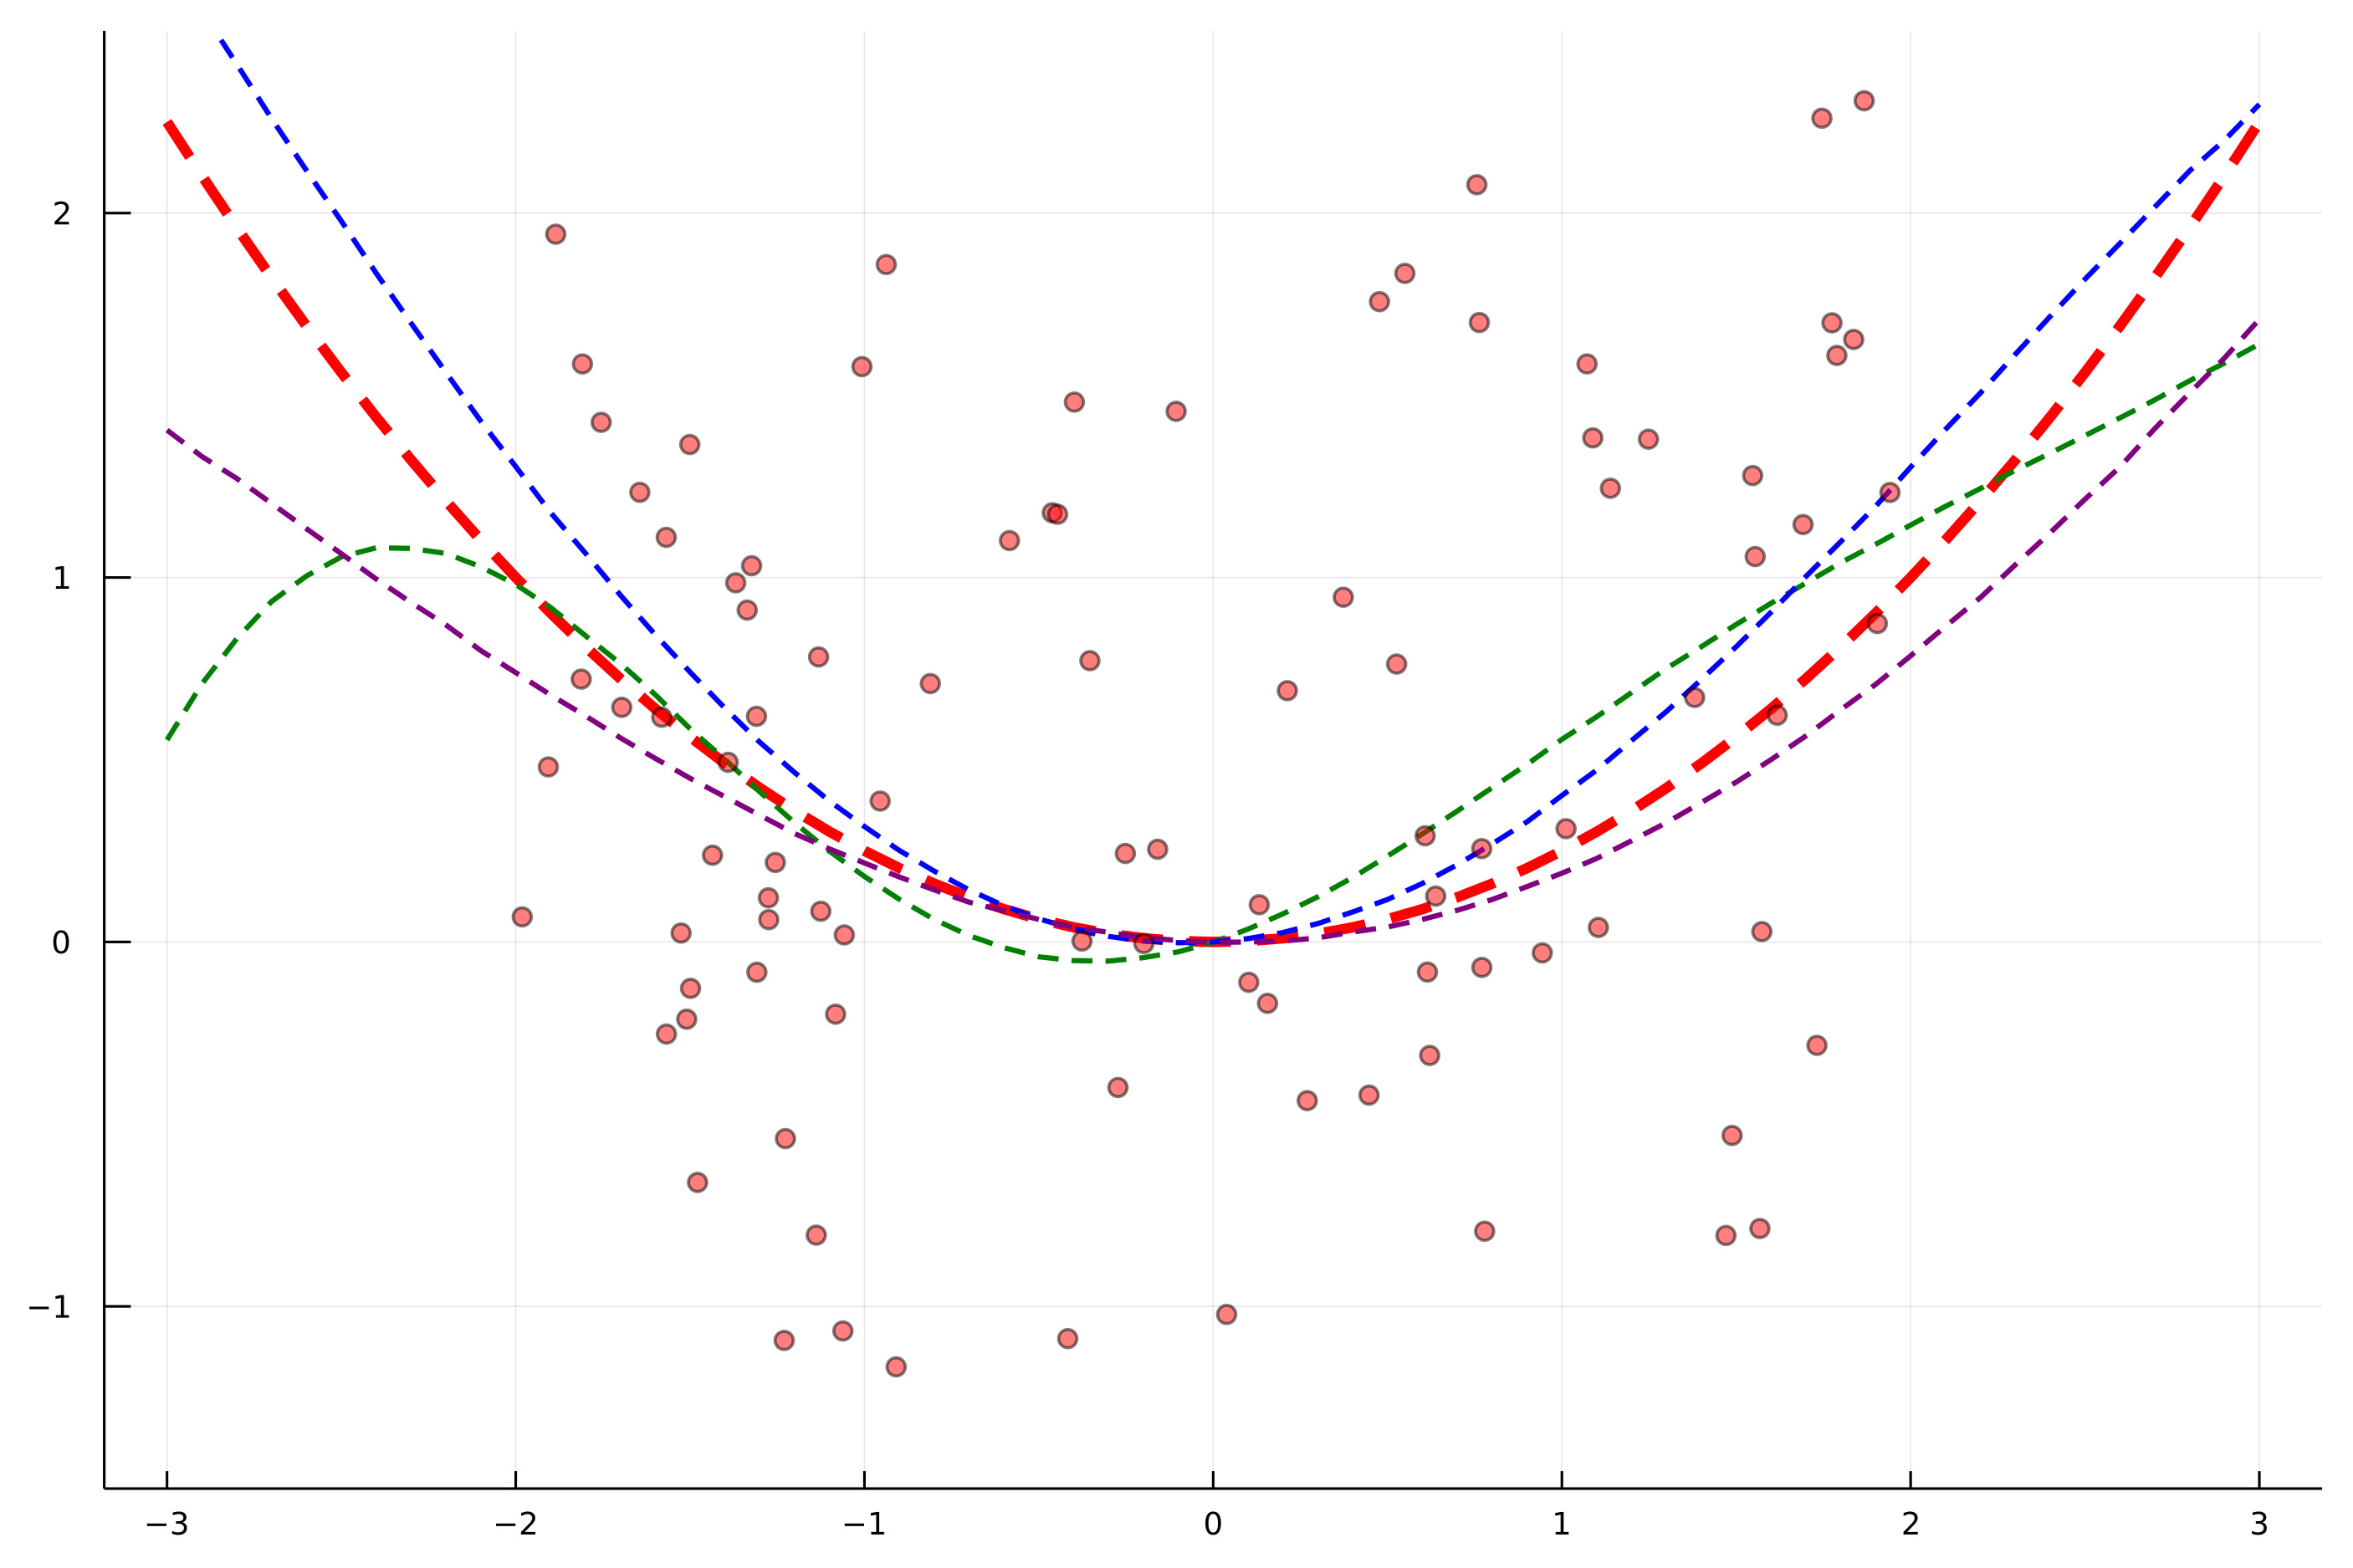}
  \label{fig:model1:sub2}
\end{subfigure}
\caption{Illustrative posterior samples for variants $4.1$ (green), $4.2$ (blue), $4.3$ (purple) for samples (red dots) of size $n_1=20$ (left) and $n_2=100$ (right) with true mean function (red).}
\label{fig:model1}
\end{figure}
